# Supplementary material for: MiniGPT4-Video: Advancing Multimodal LLMs for Video Understanding with Interleaved Visual-Textual Tokens
Source: arXiv:2404.03413 source file (2024-04-04)
Supplement: Supplementary file 1 [file X_suppl.tex]

\clearpage
\setcounter{page}{1}
\maketitlesupplementary

\section{Related work}
\label{sec:related_work}
%\subsection{Large Vision-Language Models}

% \subsection{LLM-Based Video Understanding}
Recently, vision-language models such as LLaVA~\cite{llava} have been extended to the video domain to process videos of a couple of minutes, with similar capabilities such as visual question-answering and captioning. Video-LLaMA~\cite{video-llama} and VideoChat~\cite{li2024videochat} extend the BLIP-2~\cite{blip2} architecture for video embedding extraction and both employ two streams for audio and visual signals. Video-LLaMA employs a Video Q-Former and an Audio Q-Former for the two streams, while VideoChat has a video embedder and a perception toolkit for captioning, tags, etc.
% Video-LLaMA~\cite{video-llama} and VideoChat~\cite{li2024videochat} extend the BLIP-2~\cite{blip2} architecture for video embedding extraction. Video-LLaMA has two streams for both audio and visual inputs from video, employing a Video Q-Former for analyzing temporal image sequences and an Audio Q-Former for audio signals.  Similarly, VideoChat~\cite{li2024videochat} has two streams: a video embedder and a perception toolkit, which invokes multiple models for captions, tags, subtitles, etc. These two streams are combined and input into the final LLM with the question to produce an answer. \jian{maybe summarize video-llama and videochat as two streams methods, and give a more compact description} 
On the other hand, Video-ChatGPT~\cite{videochatgpt} leverages a single stream where the architecture first encodes each frame and then has a spatial and temporal pooling process that is finally mapped to an LLM with a linear layer. Video LLaVA~\cite{video-llava} takes advantage of the LanguageBind module to map both image and video inputs to the same embedding space. Otter~\cite{li2023otter} proposed an instruction-tuned version of OpenFlamingo such that it can also process multiple video frames as input.

\section{Prompts Details}
\label{section:prompt}

\subsection{Evaluation prompts.} We followed the same evaluation setting in videochatgpt\cite{videochatgpt}. The \{question\}, \{answer\}, and \{pred\} correspond to the question, the ground truth answer, and the model prediction, respectively, in the prompt. The \textbf{System prompt} is as follows:

{\color{darkgray}
You are an intelligent chatbot designed for evaluating the correctness of generative outputs for question-answer pairs.
Your task is to compare the predicted answer with the correct answer and determine if they match meaningfully. Here's how you can accomplish the task:\\
INSTRUCTIONS: 
\begin{itemize}
    \item Focus on the meaningful match between the predicted answer and the correct answer.
    \item Consider synonyms or paraphrases as valid matches.
    \item Evaluate the correctness of the prediction compared to the answer.
\end{itemize}
User prompt:\\
Please evaluate the following video-based question-answer pair:
\begin{flushleft}
    Question: \{question\} \\
    Correct Answer: \{answer\} \\
    Predicted Answer: \{pred\}
\end{flushleft}

Provide your evaluation only as a yes/no and score where the score is an integer value between 0 and 5, with 5 indicating the highest meaningful match. Please generate the response in the form of a Python dictionary string with keys `pred' and `score', where the value of `pred' is a string of `yes' or `no' and the value of `score' is an INTEGER, not STRING. DO NOT PROVIDE ANY OTHER OUTPUT TEXT OR EXPLANATION. Only provide the Python dictionary string. For example, your response should look like this: \{`pred': `yes', `score': 4.8\}. 
}

\section{Qualitative Results}
\label{section:qual}

Here in this section we show some qualitative results for our model to show the performance of it and its ability to answer different questions.
For each example you can open the video link which attached to the figure description to watch the video.

\begin{figure}[t!]
    \centering
    \includegraphics[width=1.0\linewidth]{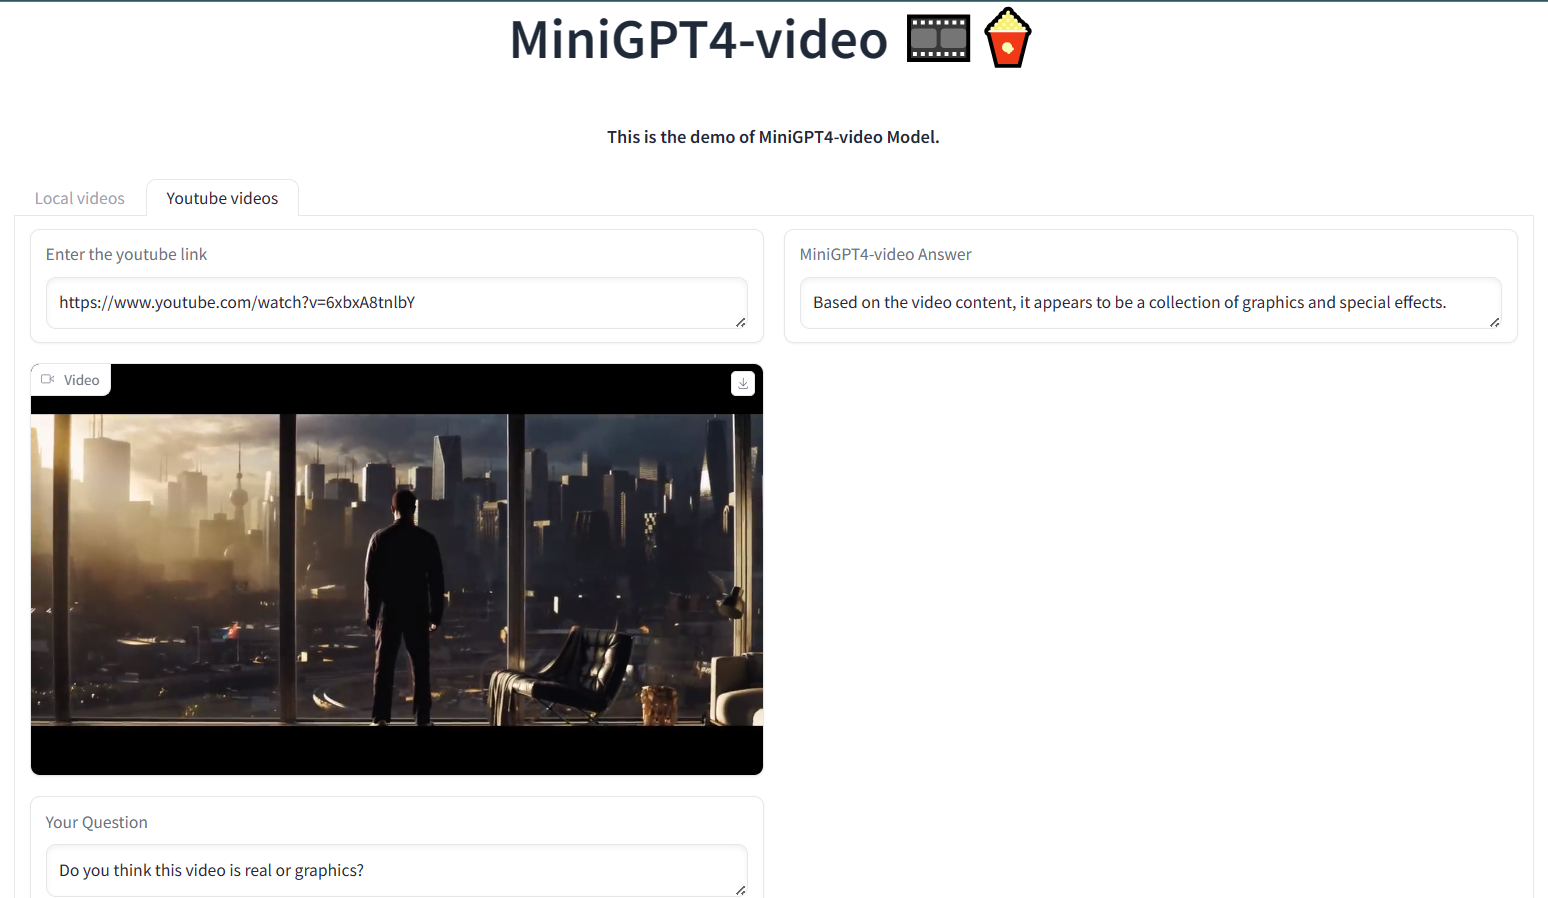}
    \captionsetup{font=scriptsize}
    \caption{Qualitative result of MiniGPT4-video for understanding general videos \href{https://www.youtube.com/watch?v=6xbxA8tnlbY&ab_channel=UnrealEngine}{[link]}.}
    \label{fig:short1}
\end{figure}

% \begin{figure}[t!]
%     \centering
%     \includegraphics[width=1.0\linewidth]{figures/4.PNG}
%     \captionsetup{font=scriptsize}
%     \caption{Qualitative result of MiniGPT4-video  understanding catron videos  \href{https://www.youtube.com/watch?v=q99eI\_uDDGc\&ab\_channel=WarnerBros.Entertainment}{[link]}.}
%     \label{fig:short2}
% \end{figure}

\begin{figure}[t!]
    \centering
    \includegraphics[width=1.0\linewidth]{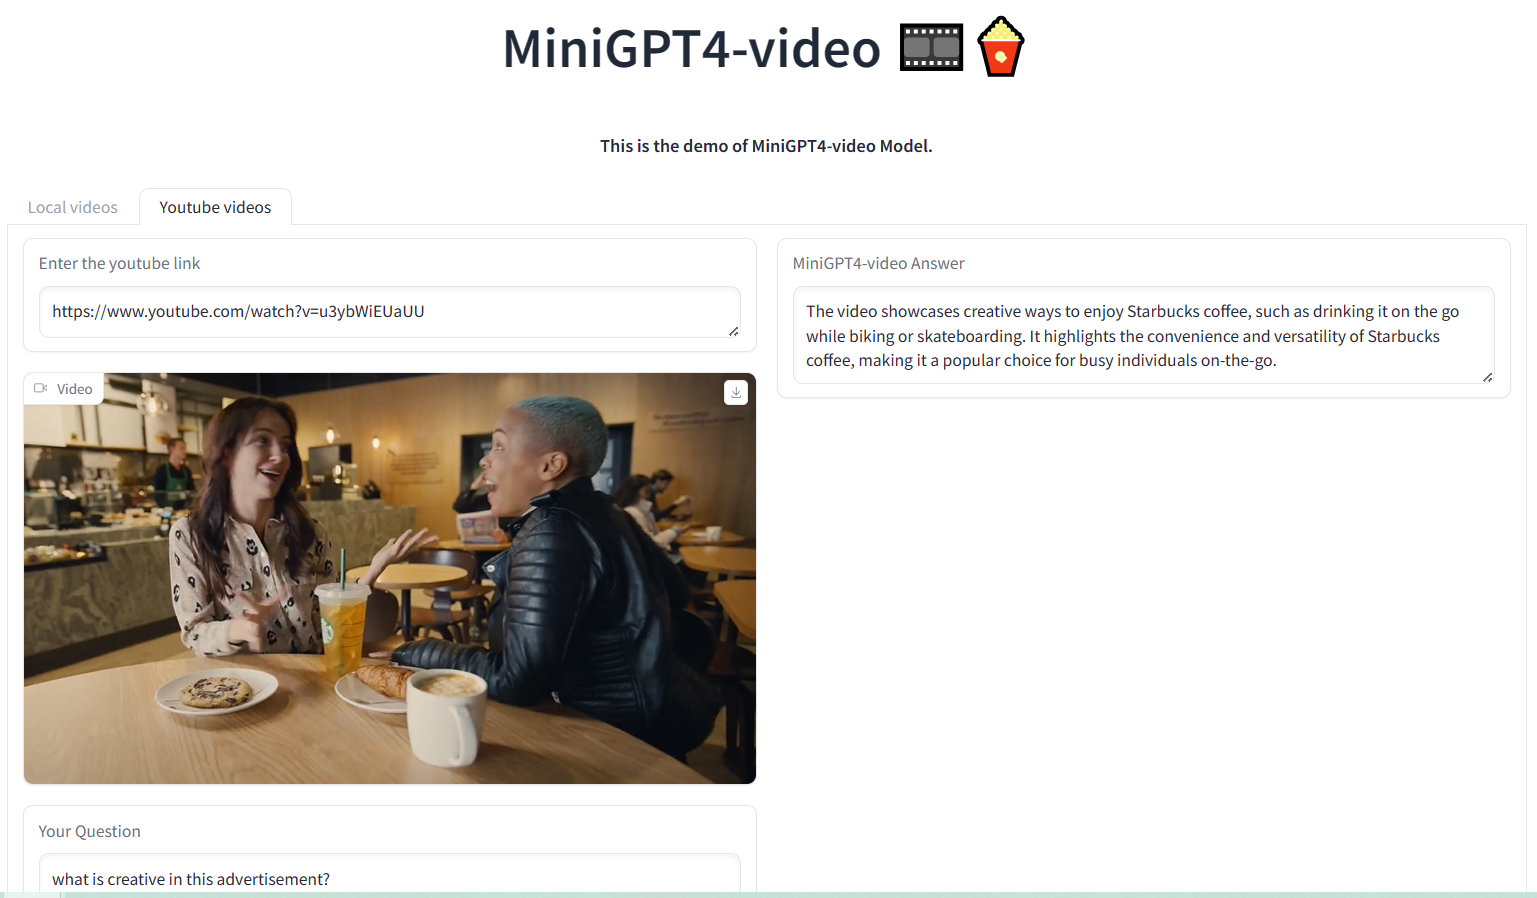}
    \captionsetup{font=scriptsize}
    \caption{Qualitative result of MiniGPT4-video  \href{https://www.youtube.com/watch?v=u3ybWiEUaUU}{[link]}.}
    \label{fig:short2}
\end{figure}

\begin{figure}[t!]
    \centering
    \includegraphics[width=1.0\linewidth]{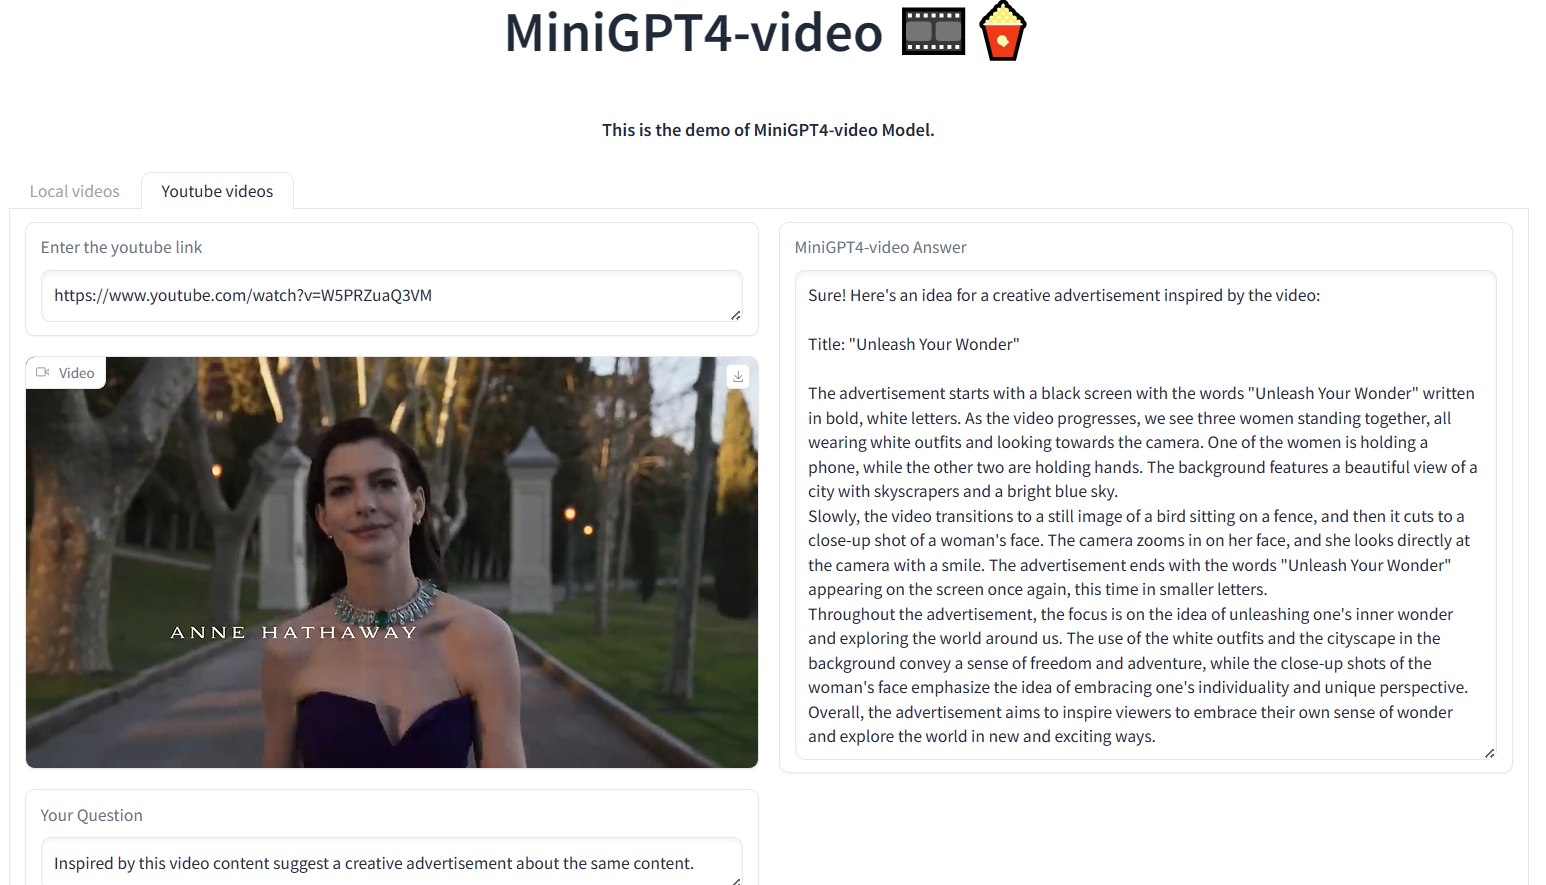}
    \captionsetup{font=scriptsize}
    \caption{Qualitative result of MiniGPT4-video  \href{https://www.youtube.com/watch?v=W5PRZuaQ3VM}{[link]}.}
    \label{fig:short2}
\end{figure}

\begin{figure}[t!]
    \centering
    \includegraphics[width=1.0\linewidth]{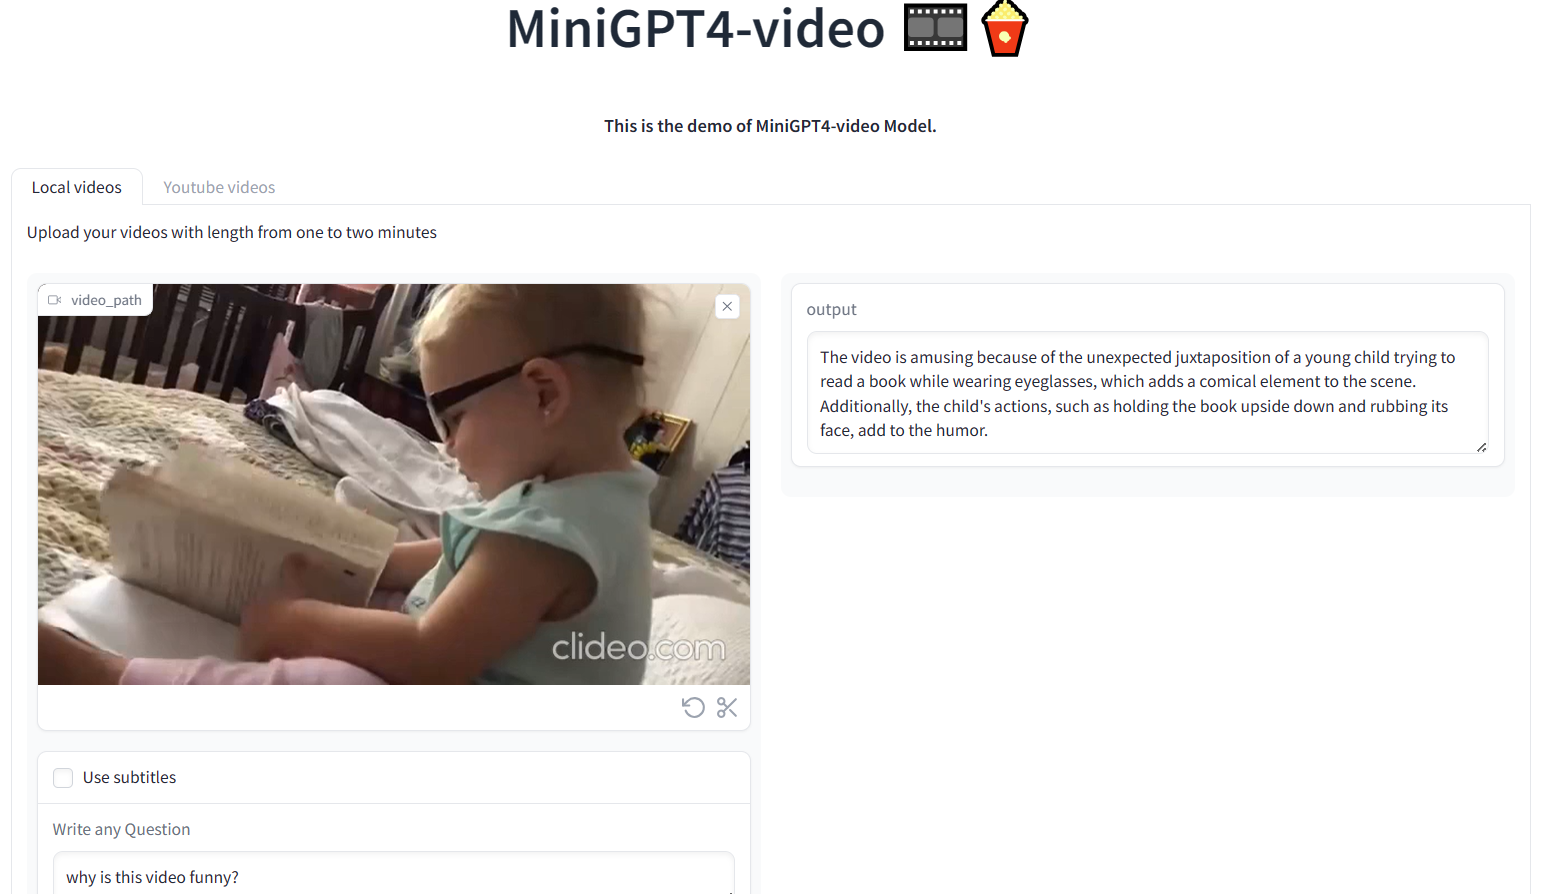}
    \captionsetup{font=scriptsize}
    \caption{Qualitative result of MiniGPT4-video}
    \label{fig:short2}
\end{figure}

\begin{figure}[t!]
    \centering
    \includegraphics[width=1.0\linewidth]{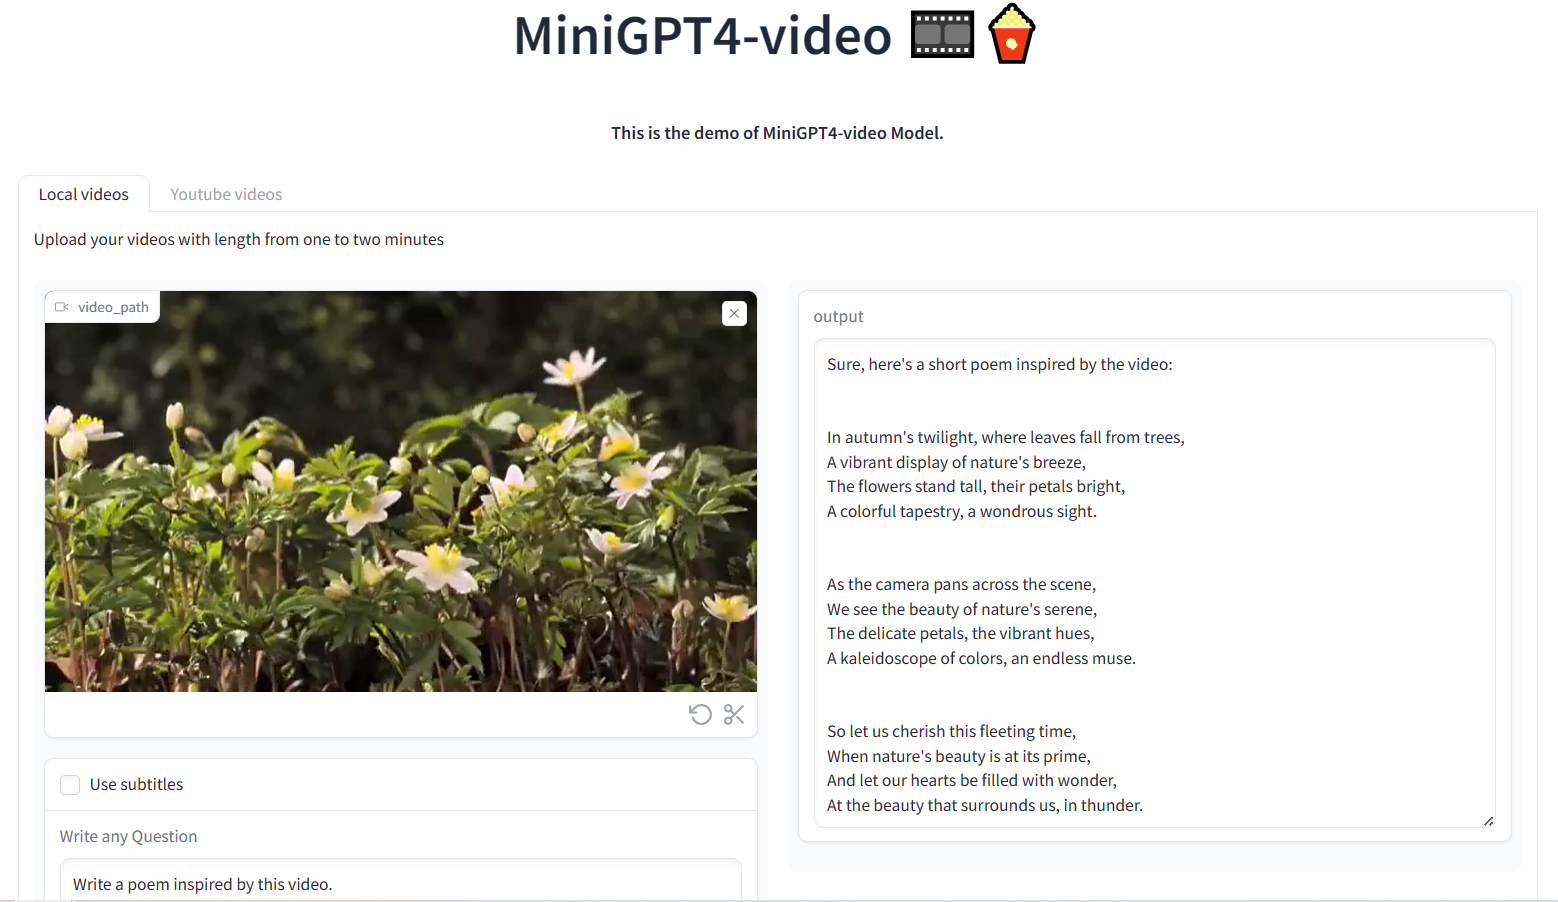}
    \captionsetup{font=scriptsize}
    \caption{Qualitative result of MiniGPT4-video}
    \label{fig:short2}
\end{figure}

\begin{figure}[t!]
    \centering
    \includegraphics[width=1.0\linewidth]{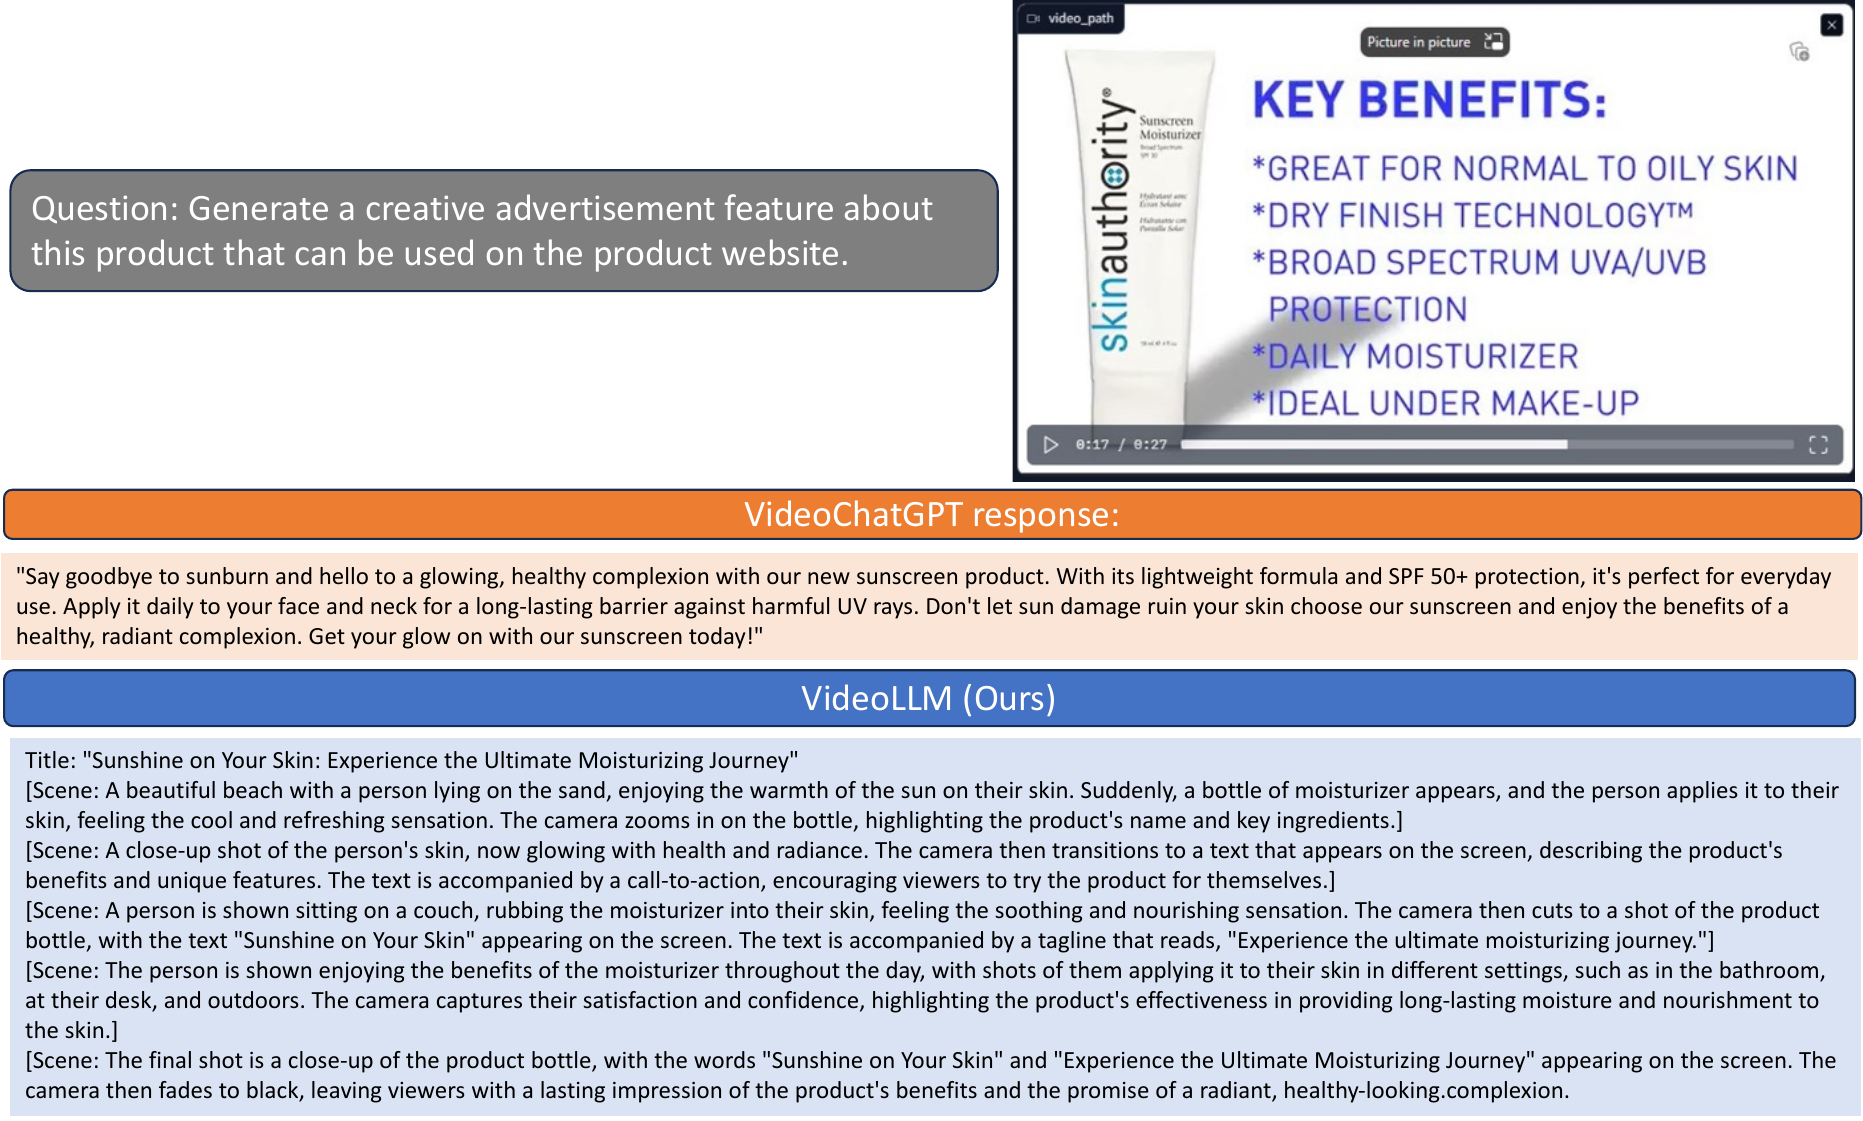}
    \captionsetup{font=scriptsize}
    \caption{\textbf{MiniGPT4-video vs VideoChatGPT~\cite{videochatgpt}.}}
    \label{fig:visionllm}
\end{figure}

\begin{figure}[t!]
    \centering
    \includegraphics[width=1.0\linewidth]{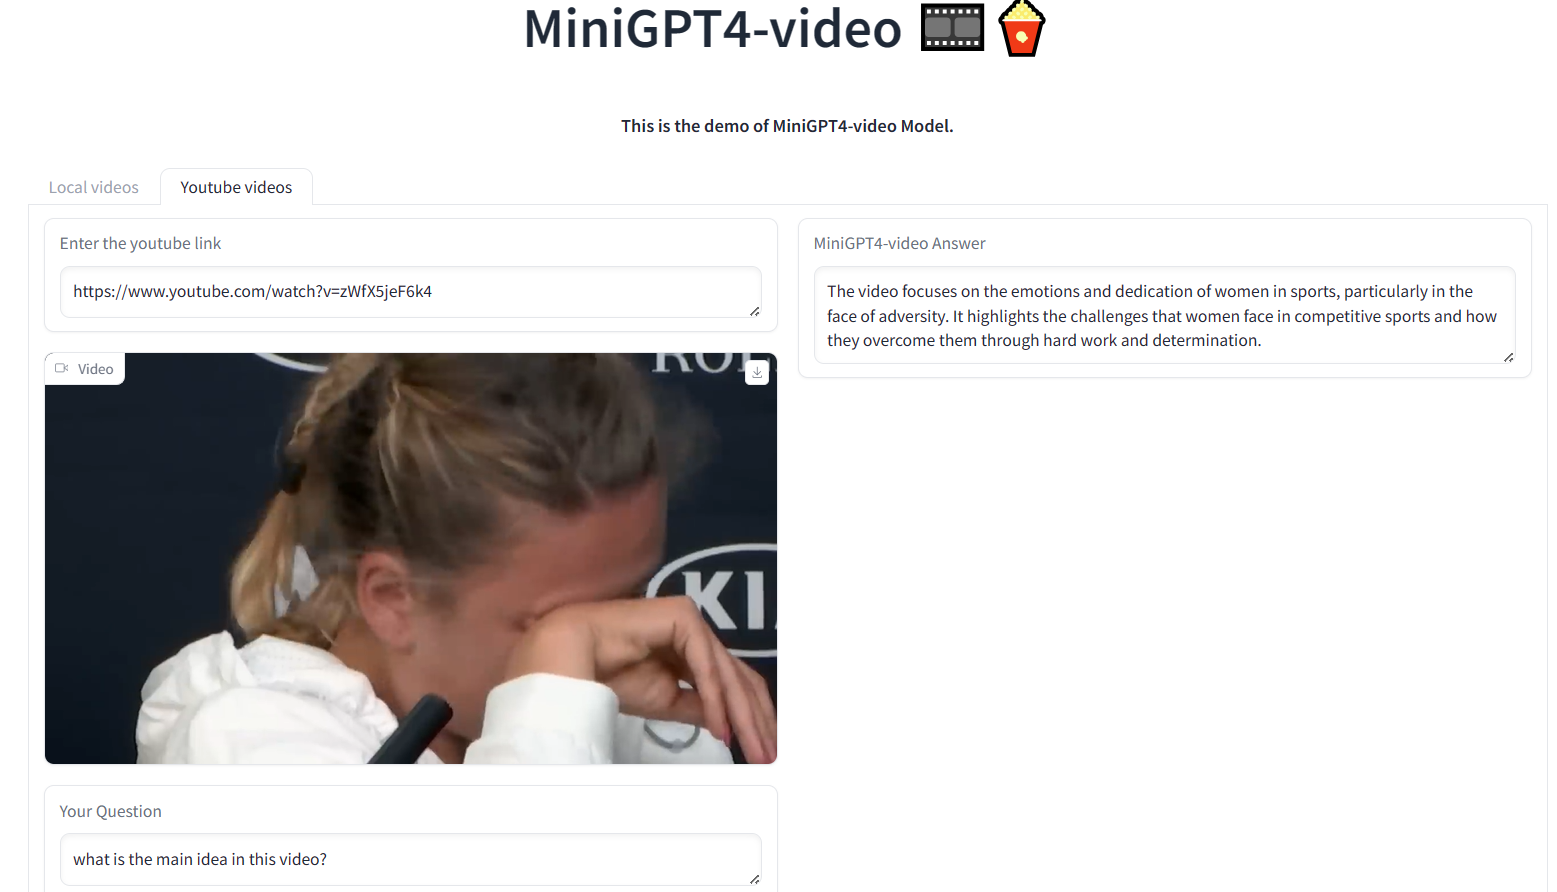}
    \captionsetup{font=scriptsize}
    \caption{Qualitative result of MiniGPT4-video \href{https://www.youtube.com/watch?v=zWfX5jeF6k4}{[link]}.}
    \label{fig:visionllm}
\end{figure}

% ----------------------------------------------
